# Supplementary material for: Innate Dynamics and Identity Crisis of a Metal Surface Unveiled by Machine Learning of Atomic Environments
Source: arXiv:2207.14622 ancillary file (2023-02-21)
Supplement: Supplementary file 1 [file SupportingInformation.pdf]

**Supporting Information for:**

# Innate Dynamics and Identity Crisis of a Metal Surface Unveiled by Machine Learning of Atomic Environments


Matteo Cioni,[1] Daniela Polino,[2] Daniele Rapetti,[1] Luca Pesce,[2] Massimo Delle Piane,[1] and Giovanni M. Pavan[1,2,a]

[1] *Department of Applied Science and Technology, Politecnico di Torino, Corso Duca degli Abruzzi 24, 10129 Torino, Italy*

[2] *Department of Innovative Technologies, University of Applied Sciences and Arts of Southern Switzerland, Polo Universitario Lugano, Campus Est, Via la Santa 1, 6962 Lugano-Viganello, Switzerland*

[a] Electronic mail: giovanni.pavan@polito.it

## S1. DETAILS ABOUT THE *NN*-POTENTIAL VALIDATION

In Table S1 are reported the values for lattice parameter, vacancy and interstitial formation energies (IFE), and surface energies. These quantities have been computed with our *NN*-potential, DFT, and the embedded atom model (EAM) of Mendelev et al[1]., and compared with available experimental data[2–4]. The setup adopted for these DFT calculations using QE is the same as described in the Methods section. First of all, the lattice parameter is calculated by optimizing the atomic positions and cell dimensions of the supercell. To calculate the vacancy formation energy, a copper atom is removed from the bulk and the remaining atoms are allowed to relax. The vacancy formation energy is then calculated using the formula:

$$E_{\mathrm{f}} = E_{\mathrm{vac}} - \left(\frac{N-1}{N}\right) E_{\mathrm{bulk}} \tag{1}$$

where $E_{\mathrm{f}}$ is the vacancy formation energy,$E_{\mathrm{bulk}}$ is the energy of the bulk, $N$ is the number of atoms in the bulk, and $E_{\mathrm{vac}}$ is the energy of the slab with one copper atom removed. To calculate the IFE, the crystal cell structure is first relaxed and the initial energy $E_0$ is calculated. Next, an atom is inserted into the relaxed structure and the system is relaxed again to obtain the final energy $E_{\mathrm{f}}^i$. Once these values are obtained, they can be used to calculate the IFE. The formula used for the calculation is:

$$E_{\mathrm{f}}^i = E_{\mathrm{f}} - \left(\frac{N+1}{N}\right) \times E_0 \tag{2}$$

Here, $E_{\mathrm{f}}^i$ is the interstitial formation energy, $E_{\mathrm{f}}$ is the total energy of the system with the interstitial atom, $E_0$ is the total energy of the perfect crystal, and $N$ is the number of atoms in the unit cell. Finally, the surface energy for each slab, including the (110) missing-row (1×2) reconstructed surface, has been calculated using the following formula:

$$\gamma = \frac{E_{\mathrm{slab}} - N_{\mathrm{slab}} E_{\mathrm{bulk}}}{2A} \tag{3}$$

where $\gamma$ is the surface energy, $E_{\mathrm{slab}}$ is the total energy of the slab, $E_{\mathrm{bulk}}$ is the total energy of bulk copper per atom, $N_{\mathrm{slab}}$ is the number of atoms in the slab, and $A$ is the surface area of the slab. Table S2 reports the adatom diffusion energy barriers (eV) computed with our trained *NN*-potential and compared with available theoretical and experimental literature data[5–14]. These quantities have been calculated by sampling about 80 diffusion events in each case at 500, 600 and 700 K. The sampled times of diffusion were then fitted

on a Poisson distribution, which provided a characteristic time for each event. The diffusion times calculated respectively at 500, 600 and 700 K: on the (100) surface were 494.8,89.73, and 27.93 ps, on the (111) 0.002,0.0017 and 0.0014 ps. On the (110) surface two paths were considered the in-channel diffusion and the cross-channel one. It is worth mentioning that the cross-channel diffusion took place always through an exchange mechanism. This is in agreement with theoretical data found in the literature. The times for these two diffusion mechanisms were found to be very close: 3.12, 7.11 and 20.5 ps for the in-channel diffusion, and 3.11, 5.55 and 23.4 ps for the cross-channel diffusion at 500, 600, and 700 K respectively in both cases. Diffusion energy barriers reported in table S2 have been calculated fitting the inverse of these times on an Arrhenius plot.

| | NN-potential | DFT | EAM | Expt. |
|---|---|---|---|---|
| lattice parameter (Å) | 3.626 | 3.630 | 3.639 | 3.615 |
| Vacancy formation (eV) | 1.14 | 1.10 | 1.07 | 1.27 |
| Interstitial formation (eV) | 3.28 | 3.49 | 3.87 | 2.8-4.2 |
| Surface energies (eV Å$^{-2}$) | | | | |
| (111) | 0.99 | 1.07 | 1.04 | 1.79[a] |
| (100) | 1.10 | 1.19 | 1.21 | 1.79[a] |
| (110) | 1.29 | 1.36 | 1.31 | 1.79[a] |
| (110)(1×2) | 1.30 | 1.38 | 1.30 | 1.79[a] |
| (211) | 1.21 | 1.28 | 1.24 | 1.79[a] |
| (210) | 1.36 | 1.50 | 1.39 | 1.79[a] |

TABLE S1. Lattice parameter, vacancy and interstitial formation energies, and surface energies computed with our trained *NN*-potential, DFT and the embedded atom model (EAM) of Mendelev et al[1]. and compared with available experimental data[2–4]. [a]For average orientation.

| Surface | NN-potential | Theory | Expt. |
|---|---|---|---|
| (100) | 0.43 | 0.39-0.53 | 0.28-0.40 |
| (110) in channel | 0.28 | 0.23-0.53 | |
| (110) cross channel | 0.31 | 0.26-0.49 | |
| (111) | 0.11 | 0.1 | 0.1-0.15 |

TABLE S2. Adatom diffusion energy barriers (eV) on Cu (100), (110), and (111) computed with our trained *NN*-potential and compared with available theoretical and experimental literature data[5–14].

In figure S1 we report the root means square testing error along the training process.

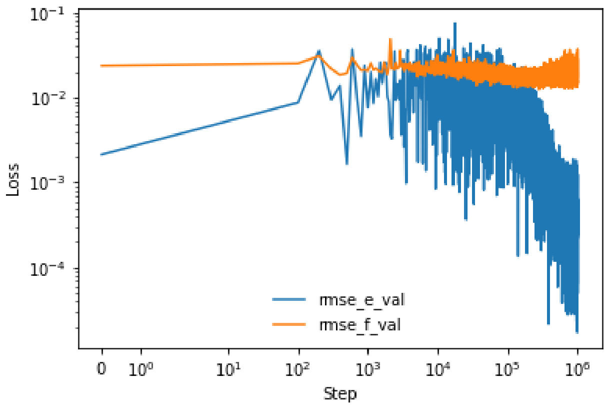


FIG. S1. **Root mean square (RMS) testing error of energy and forces during the training process**

## S2. TIME SERIES OF THE *BOTTOM-UP* SOAP CLUSTER POPULATIONS

In figures S2,S3, and S4 we report details about the populations of the SOAP clusters detected by the *bottom-up* analysis as a function of time

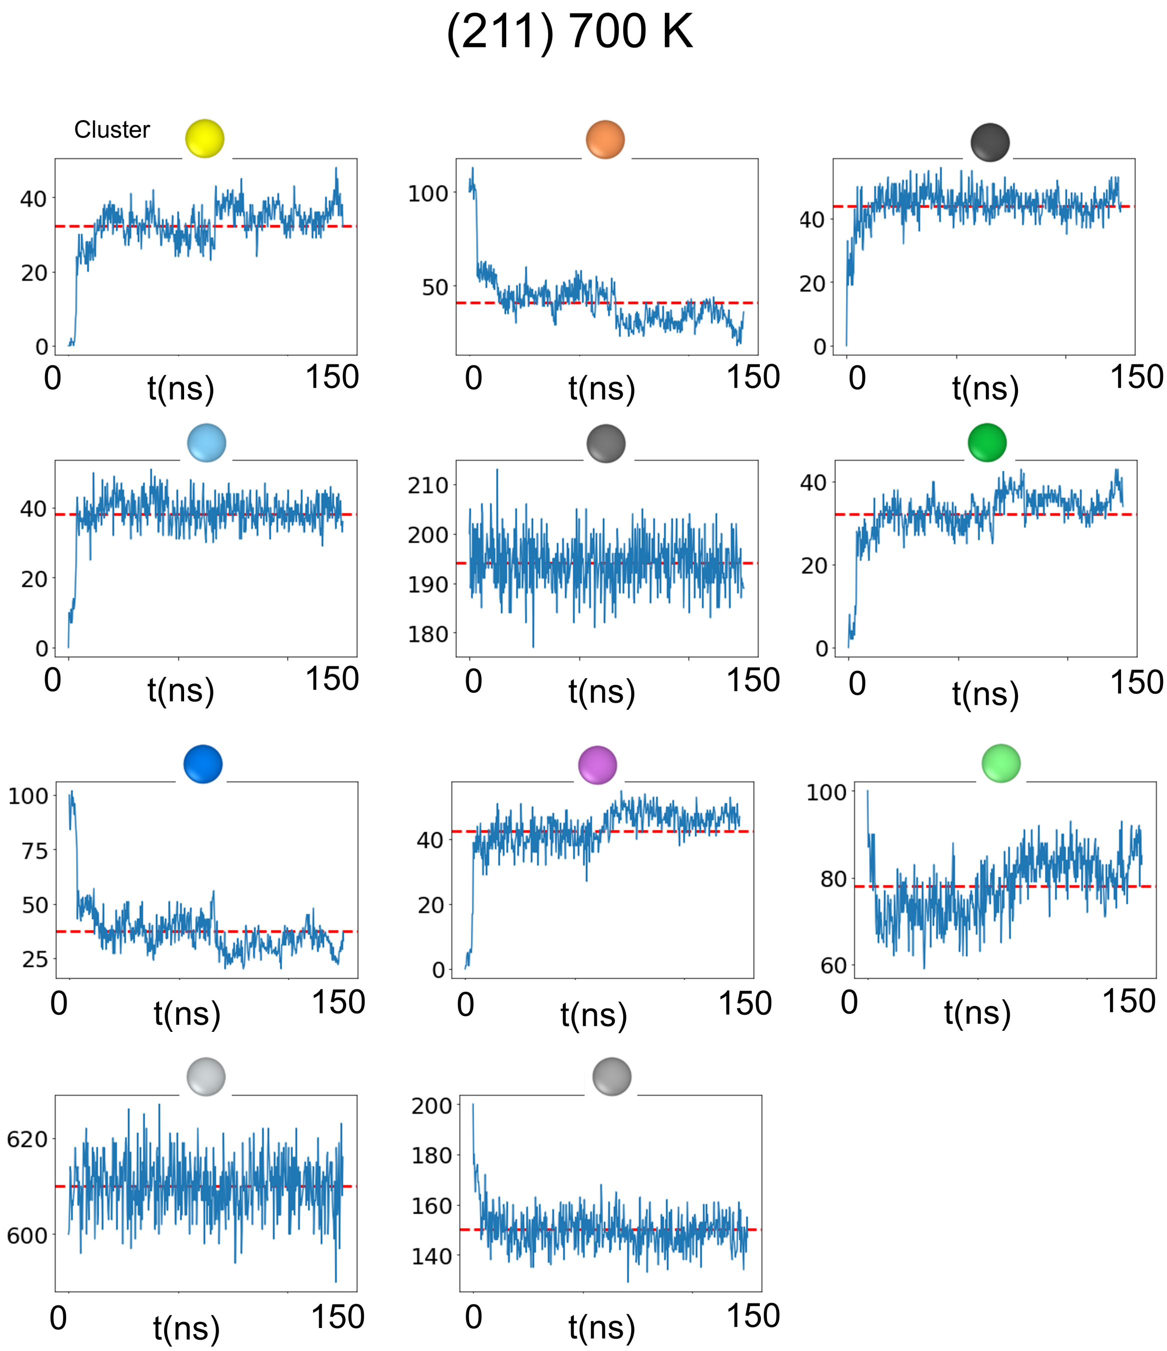


FIG. S2. Populations for the SOAP environments (number of atoms) over DPMD simulation time obtained from the *bottom-up* analysis of surface Cu(211) at 700 K described in Figure 3 in the main paper.

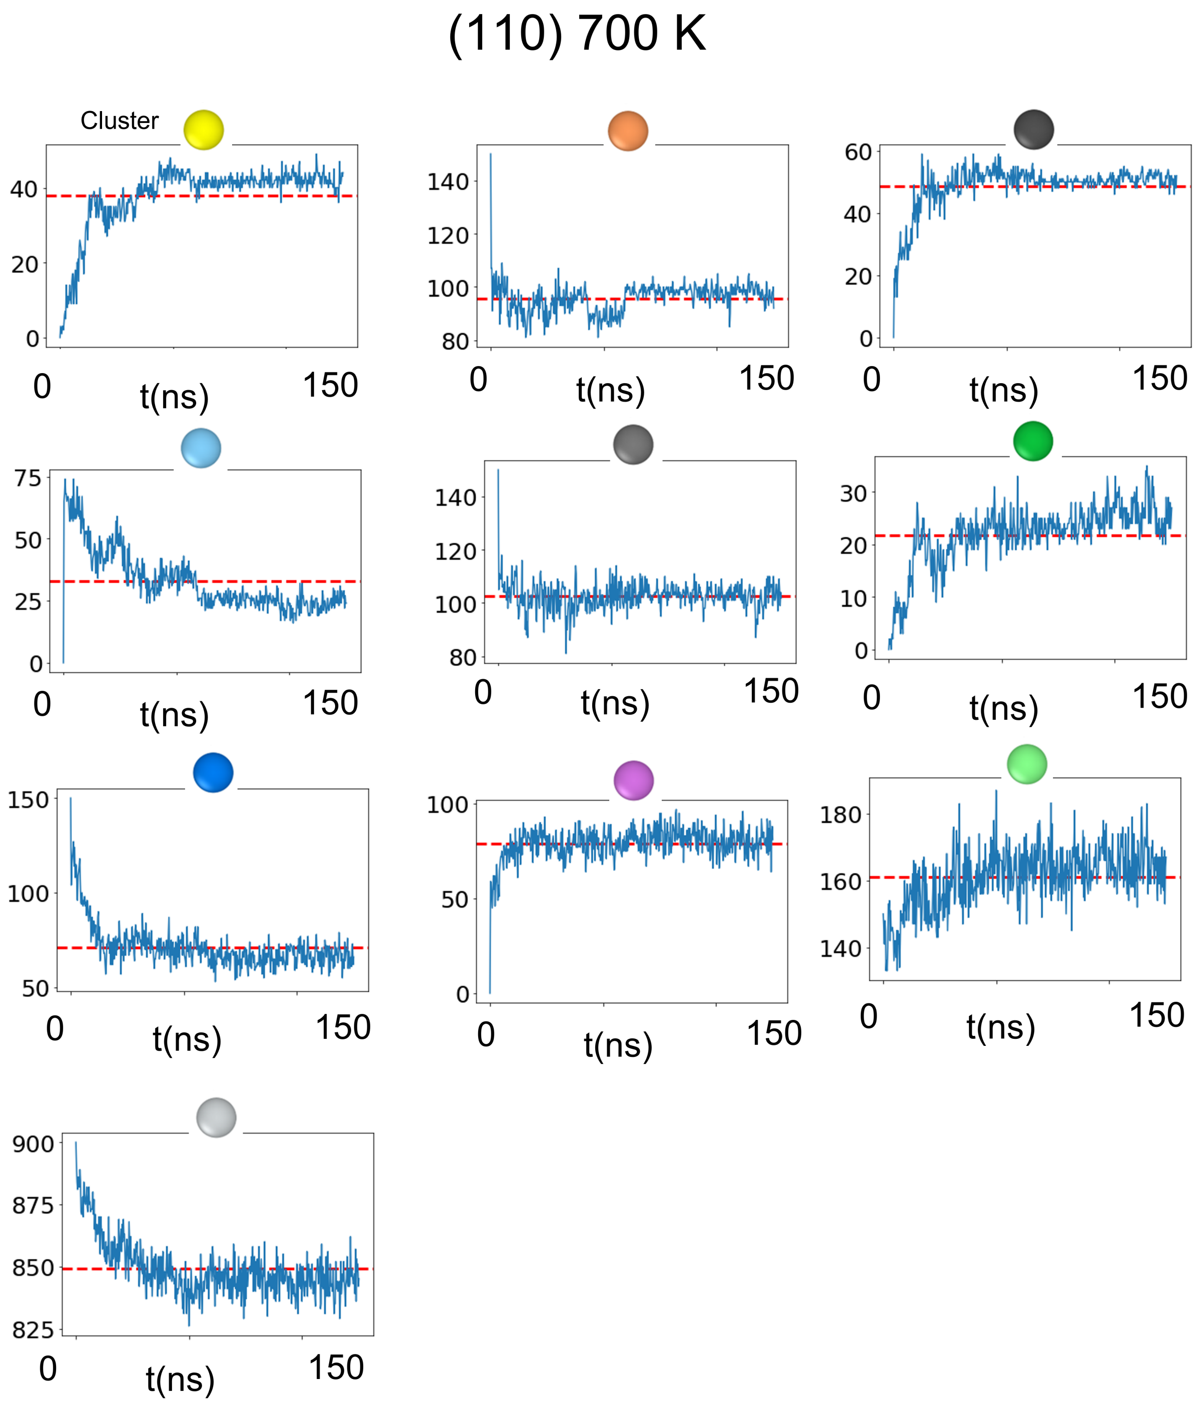


FIG. S3. Populations for the SOAP environments (number of atoms) over DPMD simulation time obtained from the *bottom-up* analysis of surface Cu(110) at 700 K described in Figure S6a-e.

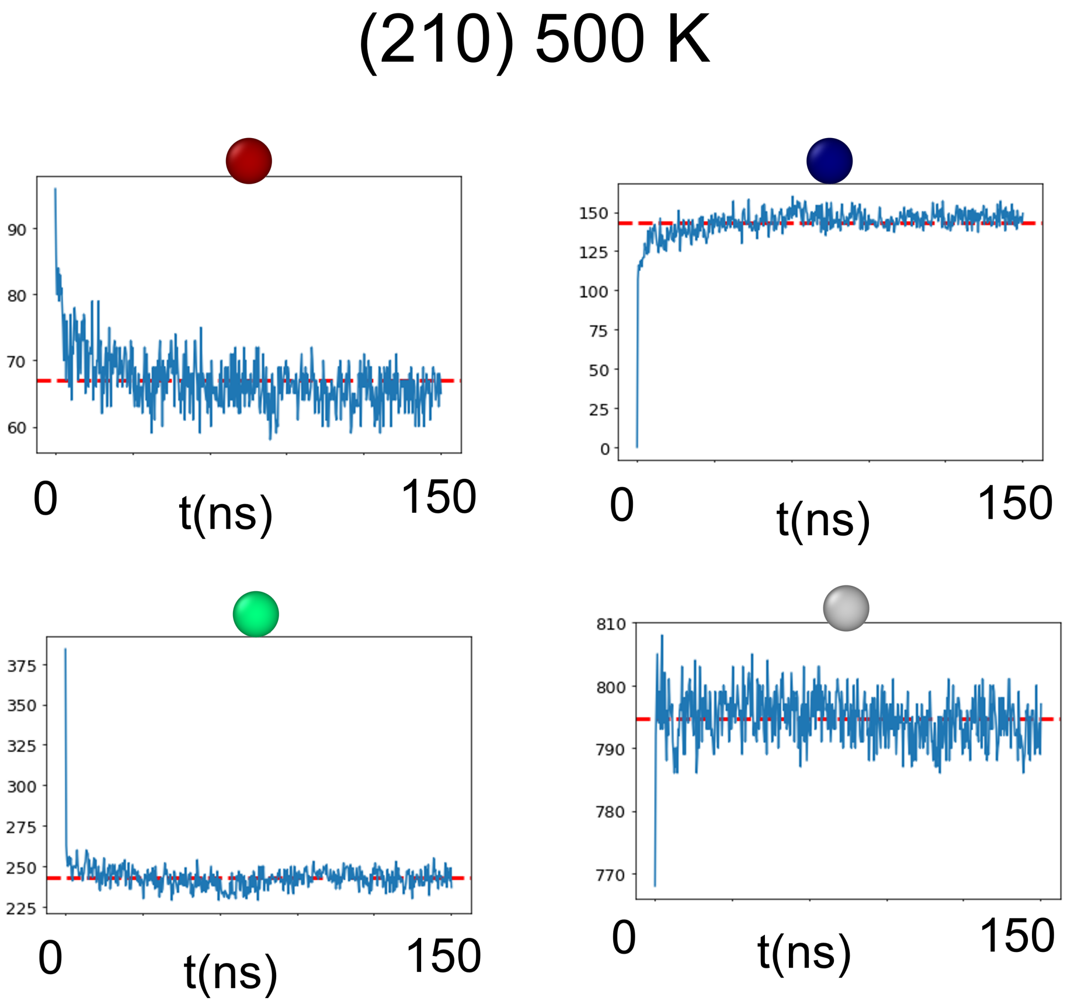


FIG. S4. Populations for the SOAP environments (number of atoms) over DPMD simulation time obtained from the *bottom-up* analysis of surface Cu(210) at 500 K described in Figure S6f-l.

## S3. ANALYSIS OF THE (110) AND (211) IDEAL MISSING-ROW TYPE RECONSTRUCTIONS

In Figures S5,S6,S7, and S8 are reported the analysis of the reconstructed (110) and (211) surfaces in order to compare their features with the results of our simulations.

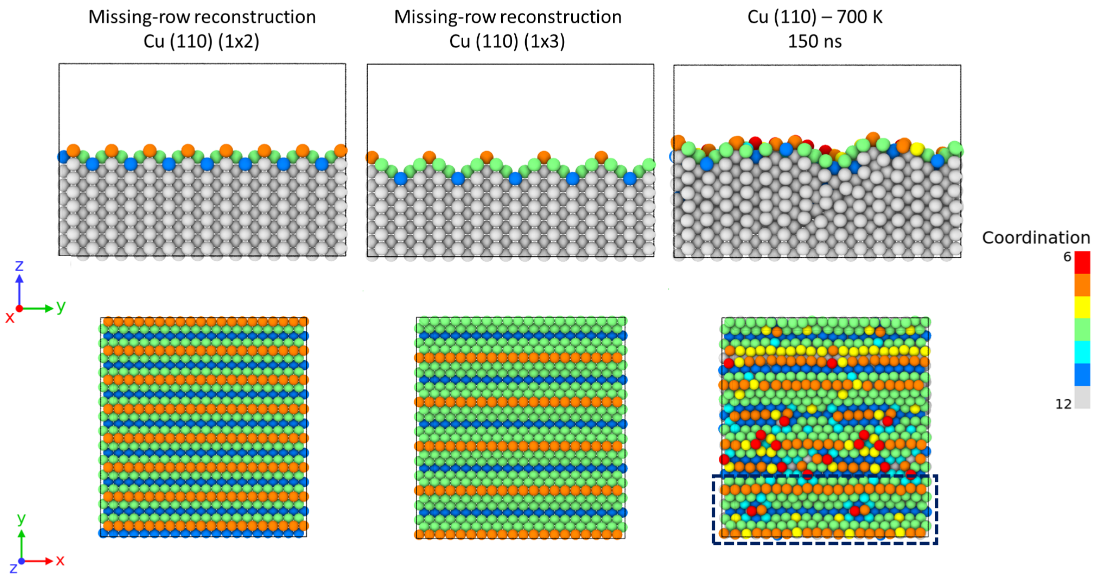


FIG. S5. Side and top views of the missing-row type reconstructions (1×2) and (1×3) for the Cu (110) surface colored according to coordination and compared with the simulated Cu (110) at 700 K after 150 ns.

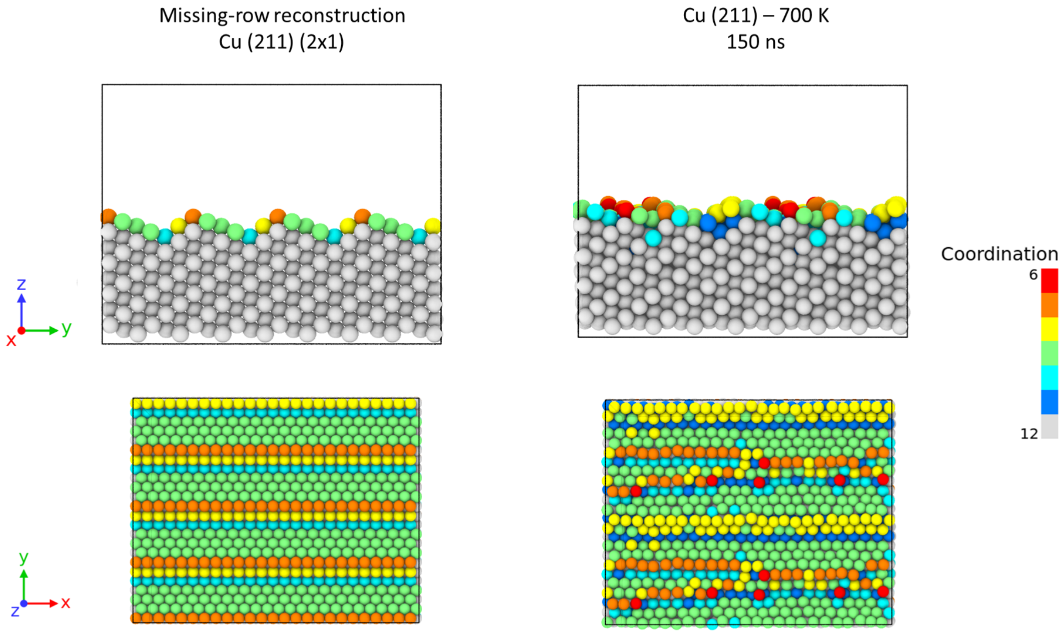


FIG. S6. Side and top views of the missing-row type reconstruction (2×1) for the Cu (211) surface colored according to coordination and compared with the simulated Cu (211) at 700 K after 150 ns.

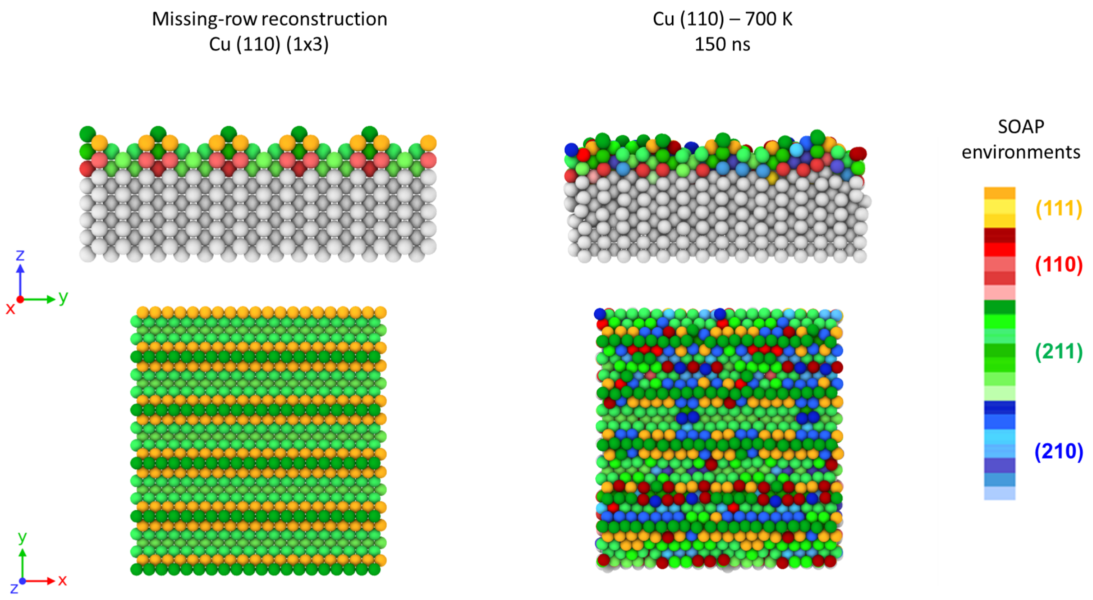


FIG. S7. Side and top views of the missing-row type reconstruction (1x3) for the Cu (110) surface colored according to the SOAP dictionary and compared with the simulated Cu (110) at 700 K after 150 ns.

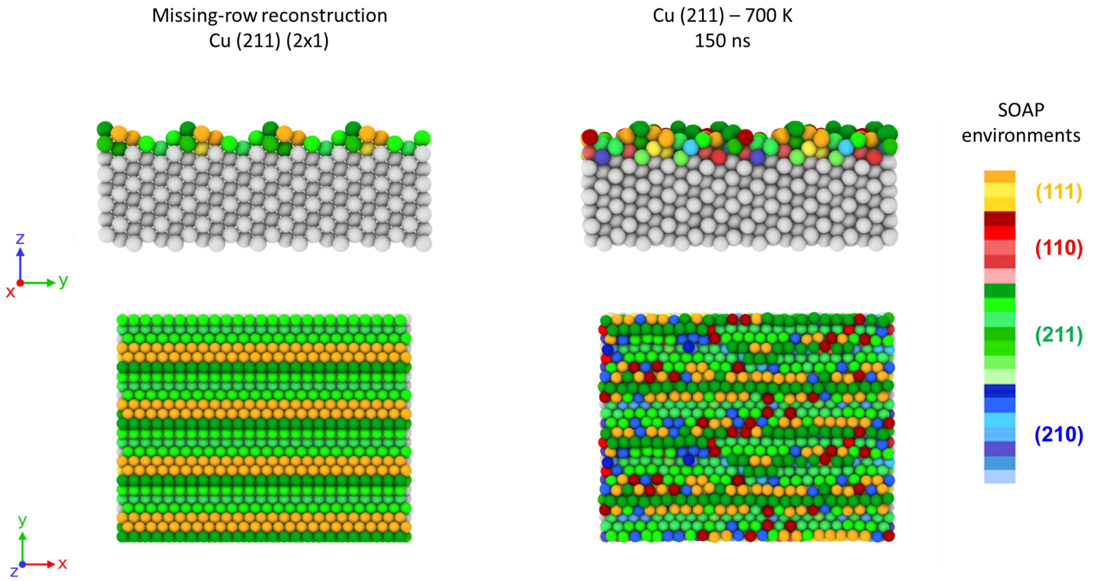


FIG. S8. Side and top views of the missing-row type reconstruction (2x1) for the Cu (211) surface colored according to the SOAP dictionary and compared with the simulated Cu (211) at 700 K after 150 ns.

## S4. RADIAL DISTRIBUTION FUNCTIONS AT DIFFERENT TEMPERATURES

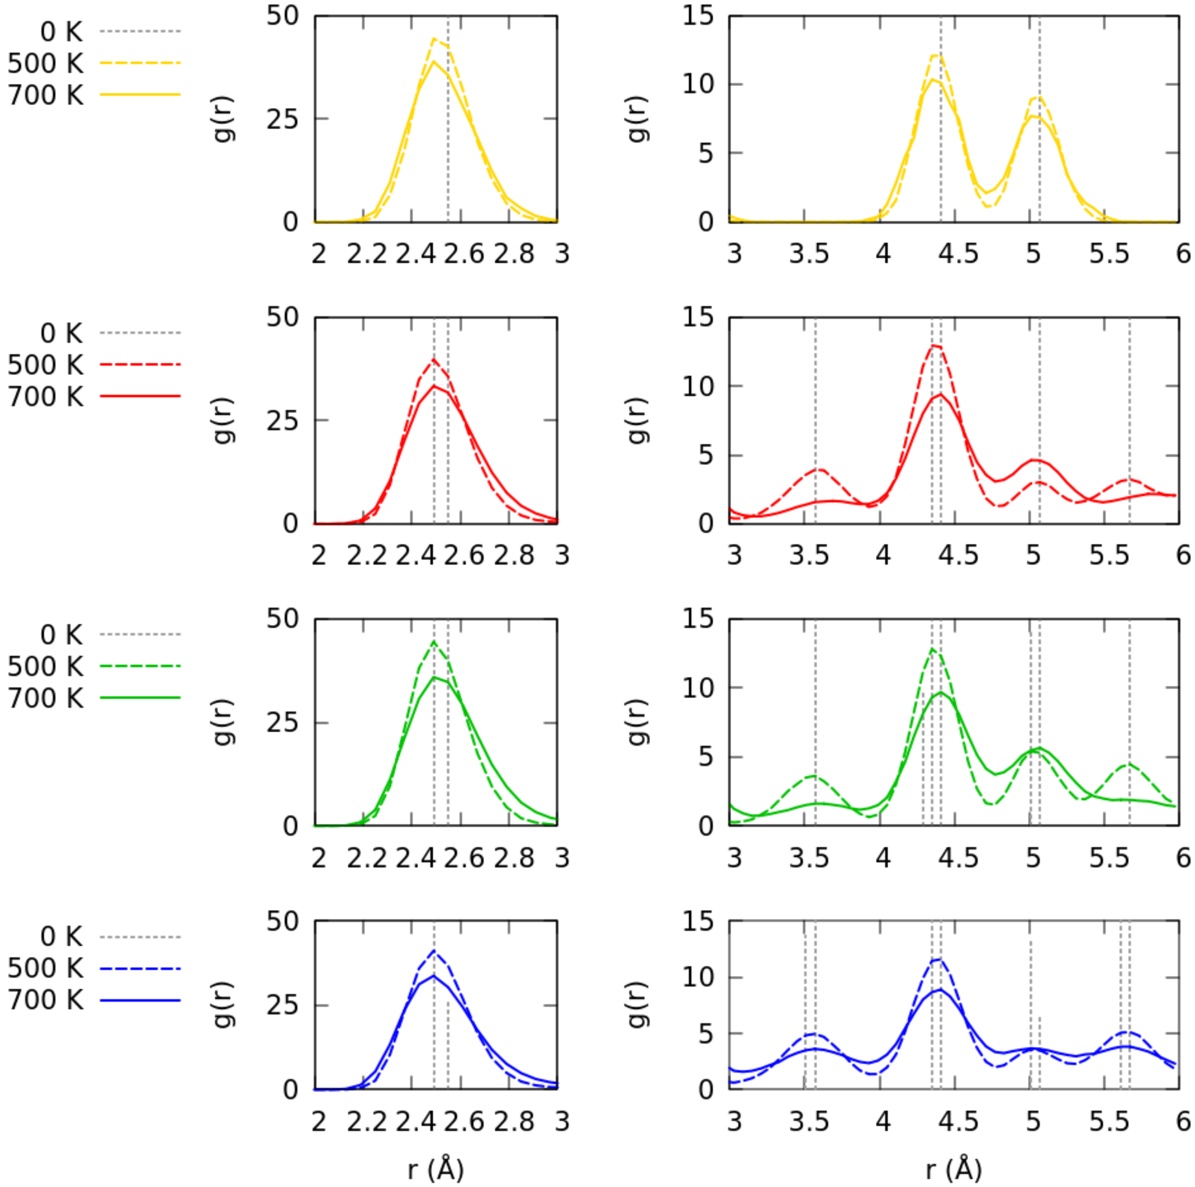


FIG. S9. Radial distribution functions of surface atoms at short (left) and longer distances (right) calculated at 0 K (with grey short-dashed impulses), at 500 (dashed lines) and 700 (solid lines) K for Cu(111) (yellow), Cu(110) (red), Cu(211) (green) and Cu(210) (blue).

## S5. ADDITIONAL DETAILS ON THE SOAP BASED ANALYSES

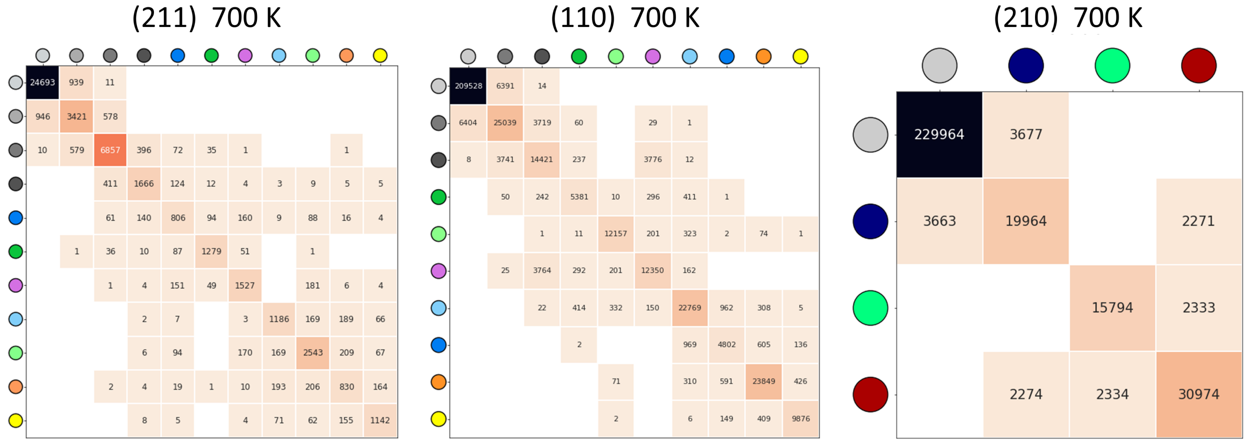


FIG. S10. Raw transition matrices obtained from counting the number of times an event is registered in $\Delta t$ for SOAP environments investigated with Unsupervised clustering (HDBSCAN*) of SOAP data for surfaces (211) at 700 K, (110) at 700 K and (210) at 500 K

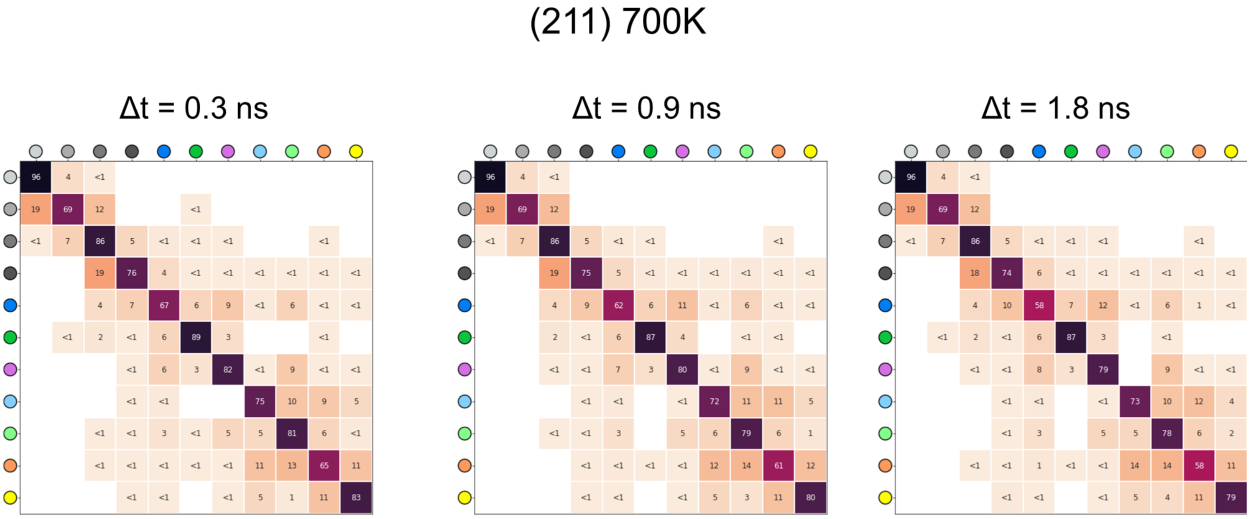


FIG. S11. Transition matrix reporting the normalized probabilities for Cu(211) at 700 K for 3 different $\Delta t$: $\Delta t = 0.3ns$, $0.9ns$ and $1.8ns$

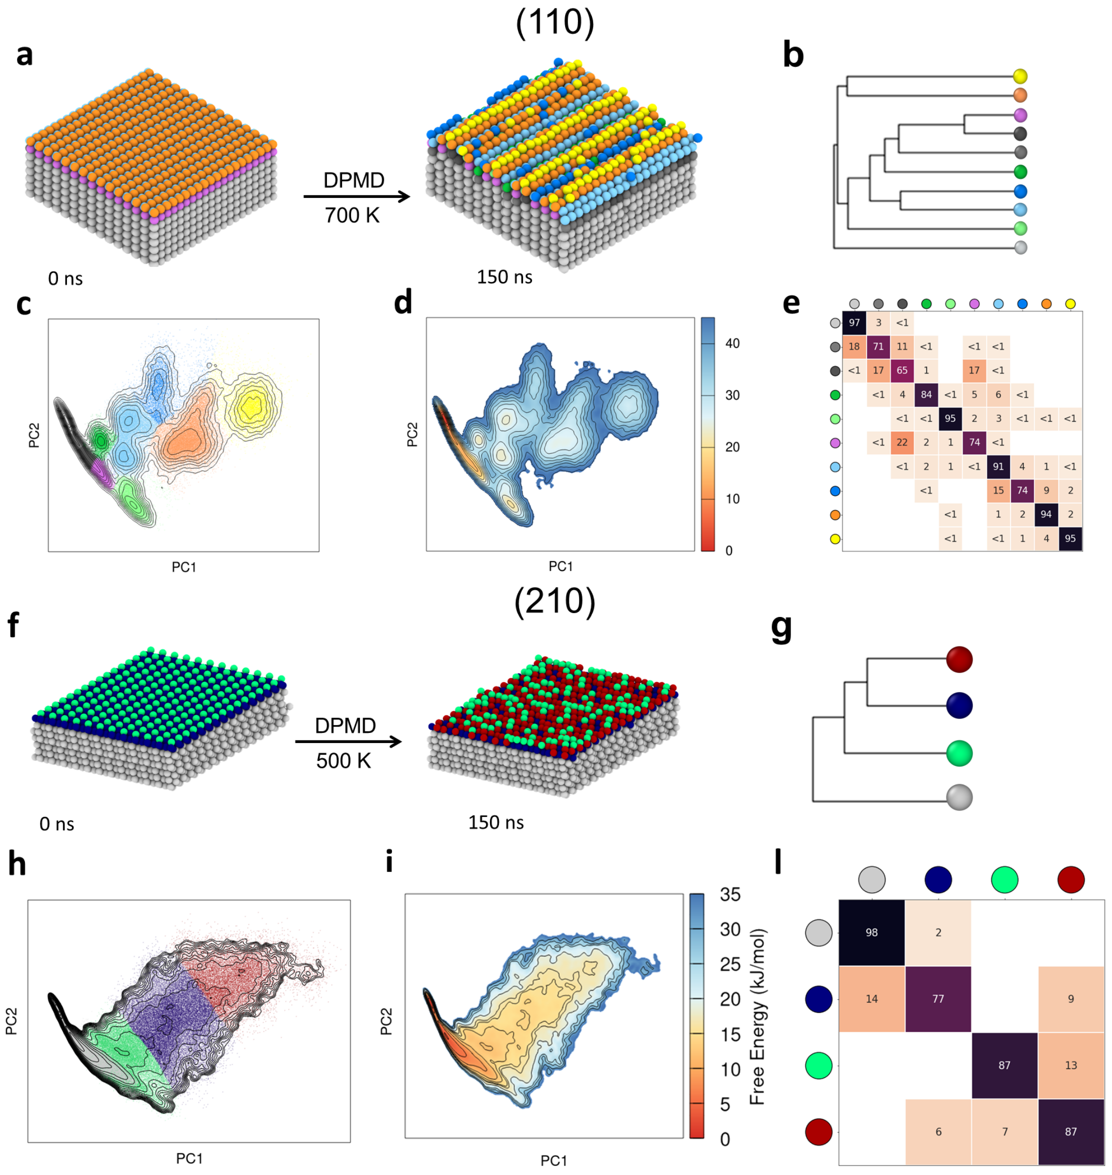


FIG. S12. ML of atomic environments in surfaces Cu(110) at 700 K and Cu(210) at 500 K and of their dynamics. **a** Cu atoms on the (110) surface colored based on the SOAP environments emerging along the equilibrium (last 75 ns) DPMD simulation at 700 K. **b** Hierarchal dendrogram connecting the 10 detected SOAP clusters. **c** Projection on the first two principal components of the SOAP data PCA with density isolines. Dots are colored according to SOAP clusters detected with HDBSCAN*. **d** Free Energy Surface (FES) computed from the PCA of the SOAP density data. **e** Transition matrix reporting the normalized probabilities (in %) for atoms to undergo a transition between the SOAP clusters in a sampling time interval of $\Delta t$ = 300 ps. **f-l** Results obtained with the same bottom-up analysis performed for surface Cu(210) at 500 K.

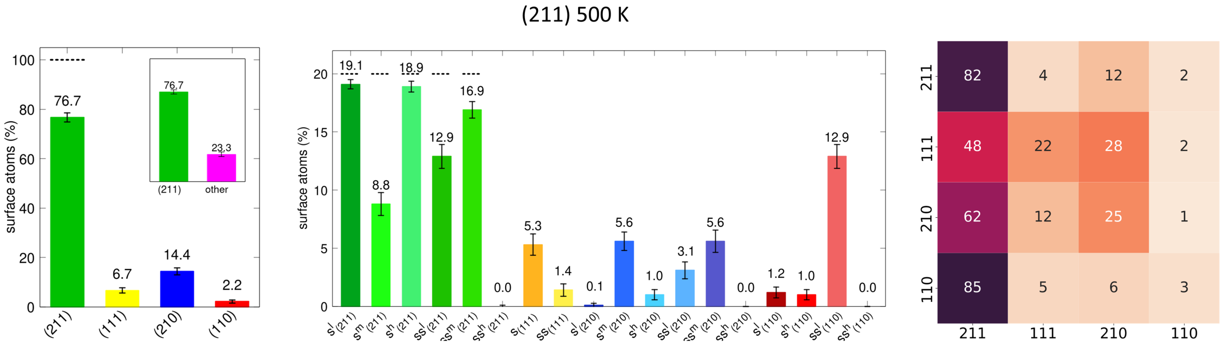


FIG. S13. **Dynamic reconstructions and equivalent identity of a Cu(211) surface at 500 K left panel** Equilibrium composition of (211) at 500 K (% and standard deviations) in terms of native (green) and non-native domains (yellow, blue, red, combined in pink in the inset). **central panel** Breakdown of (211) composition at 500 K. Dashed lines indicate the composition at DPMD start. **right panel** Transition matrix showing the probabilities for atomic transitions in (211) between native and non-native environments at 500 K (within $\Delta t = 300$ ps).

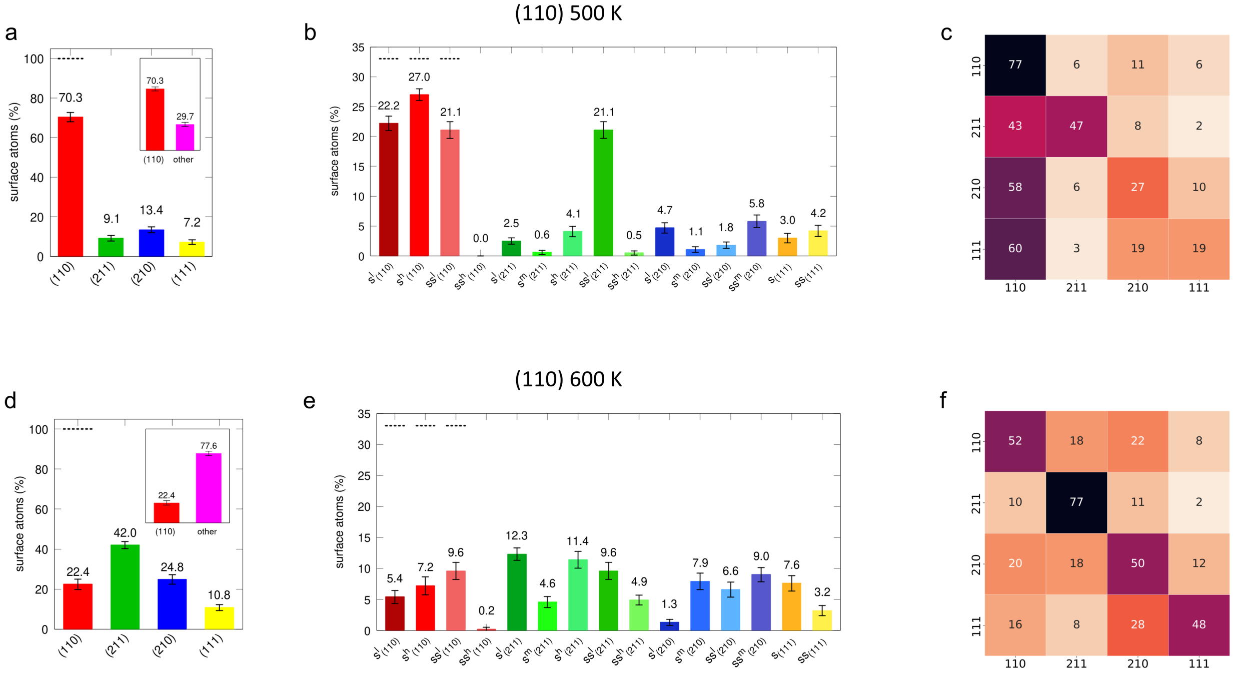


FIG. S14. **Dynamic reconstructions and equivalent identity of a Cu(110) surface at 500 K and 600 K a** Equilibrium composition of (110) at 500 K (% and standard deviations) in terms of native (red) and non-native domains (green, blue, yellow, combined in pink in the inset). **b** Breakdown of (110) composition at 500 K. Dashed lines indicate the composition at DPMD start. **c** Transition matrix showing the probabilities for atomic transitions in (110) between native and non-native environments at 500 K (within $\Delta t = 300$ ps). **d-f** Same analyses for Cu(110) at 600 K.

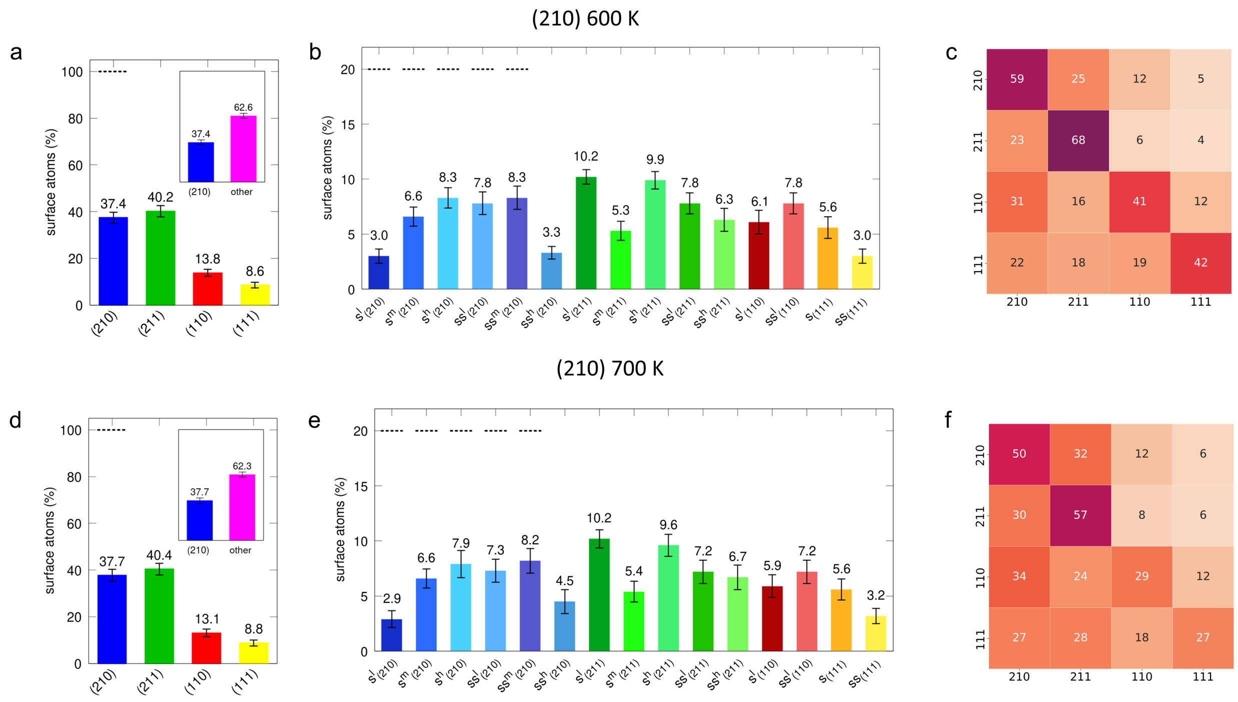


FIG. S15. **Dynamic reconstructions and equivalent identity of a Cu(210) surface at 600 K and 700 K a** Equilibrium composition of (210) at 600 K (% and standard deviations) in terms of native (blue) and non-native domains (green, red, yellow, combined in pink in the inset). **bl** Breakdown of (210) composition at 600 K. Dashed lines indicate the composition at DPMD start. **c** Transition matrix showing the probabilities for atomic transitions in (210) between native and non-native environments at 600 K (within $\Delta t = 300$ ps). **d-f** Same analyses for Cu(210) at 700 K.

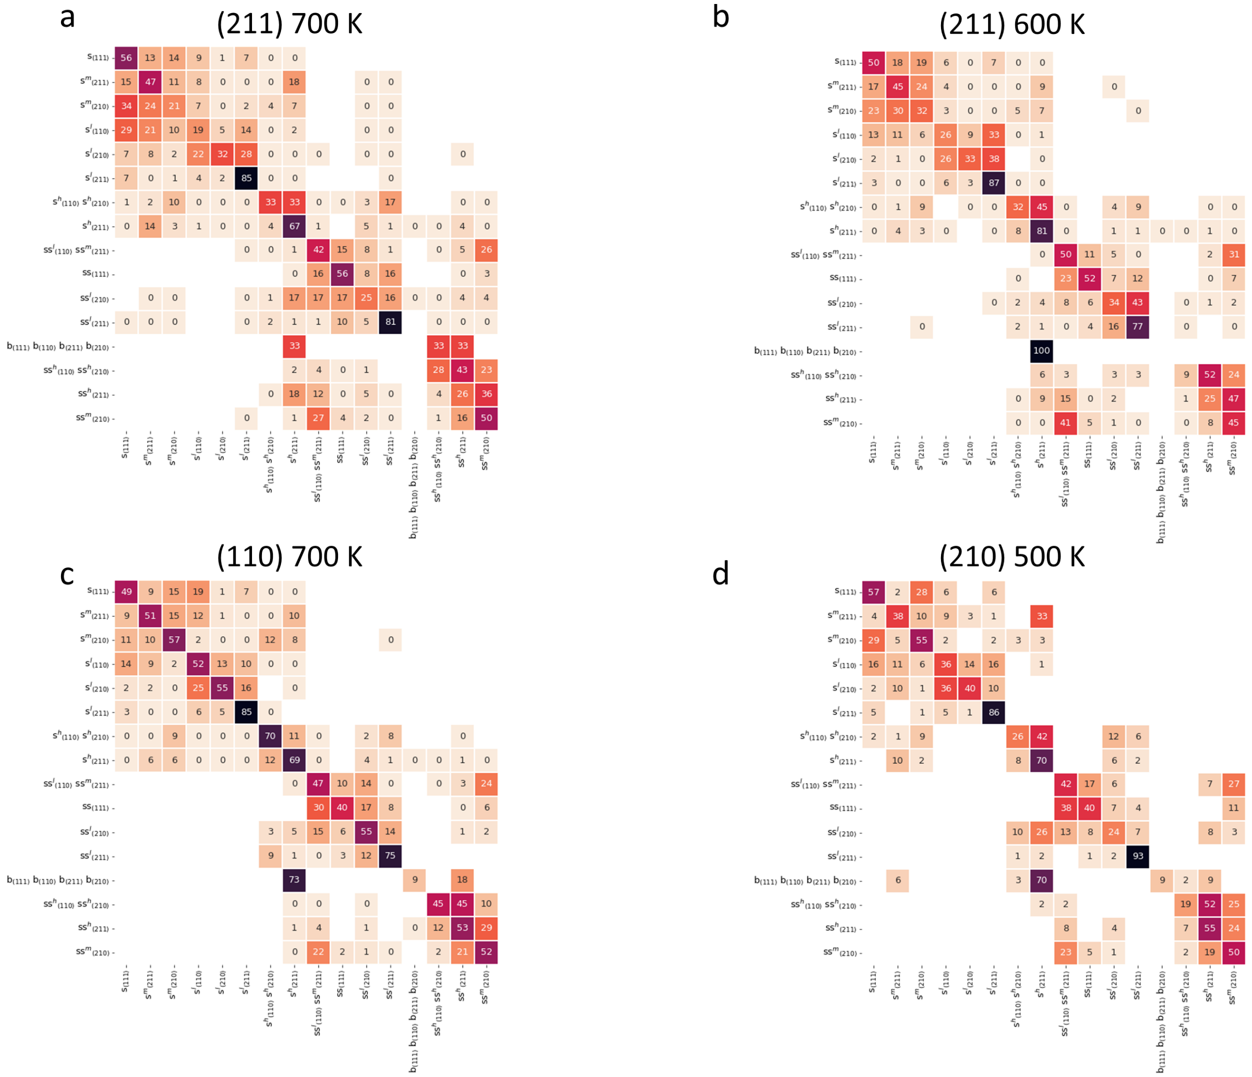


FIG. S16. **Normalized transition matrix showing the whole SOAP data-set**

## REFERENCES


[1]M. Mendelev, M. Kramer, C. Becker, and M. Asta, "Analysis of semi-empirical interatomic potentials appropriate for simulation of crystalline and liquid Al and Cu," Philos. Mag. **88**, 1723–1750 (2008).

[2]C. Kittel and P. McEuen, *Introduction to solid state physics* (John Wiley & Sons, 2018).

[3]E. A. Brandes and G. Brook, *Smithells metals reference book* (Elsevier, 2013).

[4]W. Tyson and W. Miller, "Surface free energies of solid metals: Estimation from liquid surface tension measurements," Surface Science **62**, 267–276 (1977).

[5]J. Merikoski, I. Vattulainen, J. Heinonen, and T. Ala-Nissila, "Effect of kinks and concerted diffusion mechanisms on mass transport and growth on stepped metal surfaces," Surface science **387**, 167–182 (1997).

[6]J. Merikoski and T. Ala-Nissila, "Diffusion processes and growth on stepped metal surfaces," Physical Review B **52**, R8715 (1995).

[7]L. S. Perkins and A. E. DePristo, "Self-diffusion mechanisms for adatoms on fcc (100) surfaces," Surface science **294**, 67–77 (1993).

[8]G. Boisvert and L. J. Lewis, "Self-diffusion of adatoms, dimers, and vacancies on cu (100)," Physical Review B **56**, 7643 (1997).

[9]C. Liu, J. Cohen, J. Adams, and A. Voter, "Eam study of surface self-diffusion of single adatoms of fcc metals ni, cu, al, ag, au, pd, and pt," Surface science **253**, 334–344 (1991).

[10]M. Scheffler, "Physical origin of exchange diffusion on fcc (100) metal surfaces," Physical review-series B- **56**, R15–569 (1997).

[11]H. Dürr, J. Wendelken, and J.-K. Zuo, "Island morphology and adatom energy barriers during homoepitaxy on cu (001)," Surface science **328**, L527–L532 (1995).

[12]H.-J. Ernst, F. Fabre, and J. Lapujoulade, "Nucleation and diffusion of cu adatoms on cu (100): A helium-atom-beam scattering study," Physical Review B **46**, 1929 (1992).

[13]L. Hansen, P. Stoltze, K. W. Jacobsen, and J. K. Nørskov, "Self-diffusion on copper surfaces," Phys. Rev. B **44**, 6523–6526 (1991).

[14]F. Montalenti and R. Ferrando, "Jumps and concerted moves in cu, ag, and au (110) adatom self-diffusion," Physical Review B **59**, 5881 (1999).
